# Supplementary material for: Estimating & Mitigating the Impact of Acoustic Environments on Machine-to-Machine Signalling
Source: arXiv:1908.04672 source file (2019-08-13)
Supplement: Supplementary file 1 [file appendix.tex]

\onecolumn
\appendices
\section{Real vs Simulated Environment Performance of Chirp Decoder} 
Before we propose the dereverberation strategy, it is necessary to obtain the empirical baseline performance of the Chirp packet decoder for different acoustic environments.
Analysing the Chirp signal decode rate when played through an environment is a time-consuming process, considering the number of environments required for the baseline performance data.
Hence, we obtained 590 RIR from the AcouSP Database  \cite{acousp}, and simulated the environment by convolving 100 packets with each RIR. Before proceeding with our main evaluation, we first performed a pilot study to validate whether the decode rate of a Chirp signal transmitted in real environment can be simulated using IRs.
Three lecture halls from Queen Mary University of London campus with varying dimensions were chosen. Two iPhone 5Cs, one transmitting and one receiving, were placed 3m apart at the centre of the room in two positions, one with the speaker and microphone facing each other and another with them facing away from each other. 200 (100 audible and 100 near-ultrasonic) packets were transmitted to the receiver and the detection of preamble tones and the payload decode was recorded. 
The performance of the Chirp decoder for real environment versus the simulated environment are shown in Table III. From the results, it can be seen that the performance of the Chirp decoder in the simulated environment is within 3\% of that of the real world. 

\begin{table}[ht]
\centering
\begin{tabular}{|c|c|c|c|}
\hline
\textbf{\begin{tabular}[c]{@{}c@{}}Room \\ and its \\ Volume\end{tabular}} & \textbf{\begin{tabular}[c]{@{}c@{}}Chirp Signal\\ Protocol\end{tabular}} & \textbf{\begin{tabular}[c]{@{}c@{}}Real \\ Environment \\ Decode Rate\\ (\%)\end{tabular}} & \textbf{\begin{tabular}[c]{@{}c@{}}Simulated \\ Environment \\ Decode Rate \\ (\%)\end{tabular}} \\ \hline
\textbf{QM GC601} & Audible & 77 & 77 \\ \cline{2-4} 
495 $m^3$ & Inaudible & 100 & 100 \\ \hline
\textbf{QM BR 4.02} & Audible & 64 & 67 \\ \cline{2-4} 
216 $m^3$ & Inaudible & 100 & 100 \\ \hline
\textbf{QM GC102} & Audible & 62 & 60 \\ \cline{2-4} 
99 $m^3$ & Inaudible & 100 & 100 \\ \hline
\end{tabular}
\caption{Real vs Simulated Environment performance of Chirp decoder}
\end{table}

\section{Spectral Gain Function}
Figure below shows a short-term spectrum of the final gain function that is obtained after the modifications.
\begin{figure}[ht]
  \centering
  \includegraphics[height=8cm]{images/gain.png}
  \caption{Spectrogram of the spectral gain function.}
  \label{fig:gainfunction}
\end{figure}
